# Supplementary material for: Towards Human Computable Passwords
Source: arXiv:1404.0024 source file (2016-09-09)
Supplement: Supplementary file 1 [file Appendix.tex]

%\end{table}
